# Supplementary material for: DA-Transformer: Distance-aware Transformer
Source: arXiv:2010.06925 source file (2021-04-11)
Supplement: Supplementary file 1 [file supplement.tex]

\section*{Supplementary Materials}

\subsection*{Ablation Study}
In this section, we present several ablation studies on using our DA-Transformer at different levels on the \textit{Amazon} and \textit{MIND} datasets. 
The results are respectively presented in Tables~\ref{ab.result} and \ref{ab.result2}.
The results show the effectiveness of the DA-Transformer at different levels.

\begin{table}[!h]
\resizebox{1\linewidth}{!}{
\begin{tabular}{lcc}
\hline
\multicolumn{1}{c}{Methods}                                  & Accuracy        & Macro-F       \\ \hline
Transformer                                           &   65.15             & 42.14                   \\
+Word DA-Transformer                       & 65.92                              & 43.76                       \\
+Sentence DA-Transformer                                & 65.85                              & 43.55                   \\  
DA-Transformer                                      &  \textbf{66.38}             & \textbf{44.29}         \\ \hline
\end{tabular}
}
 \caption{Results on the \textit{Amazon} dataset.}
\label{ab.result}
\end{table}

\begin{table}[!h]
\resizebox{1\linewidth}{!}{
\begin{tabular}{lcccc}
\hline
\multicolumn{1}{c}{\textbf{Methods}} & AUC                                & MRR                                & \small{nDCG@5}                             & \small{nDCG@10}        \\ \hline
Transformer                      & 67.81                              & 33.10                              & 35.98                              & 41.65          \\
+Word DA-Transformer                       & 68.10                              & 33.21                              & 36.19                              & 42.07          \\
+News DA-Transformer                                & 68.24                              & 33.30                              & 36.29                              & 42.01          \\ \hline
+Both                     & \textbf{68.32} & \textbf{33.36} & \textbf{36.34} & \textbf{42.07} \\ \hline
\end{tabular}
}
 \caption{Results on the \textit{MIND} dataset.}
\label{ab.result2}
\end{table}

\subsection*{Additional Experimental Results}

\begin{figure}[!h]
	\centering 
	\subfigure[\textit{SST}.]{
	\includegraphics[height=1.5in]{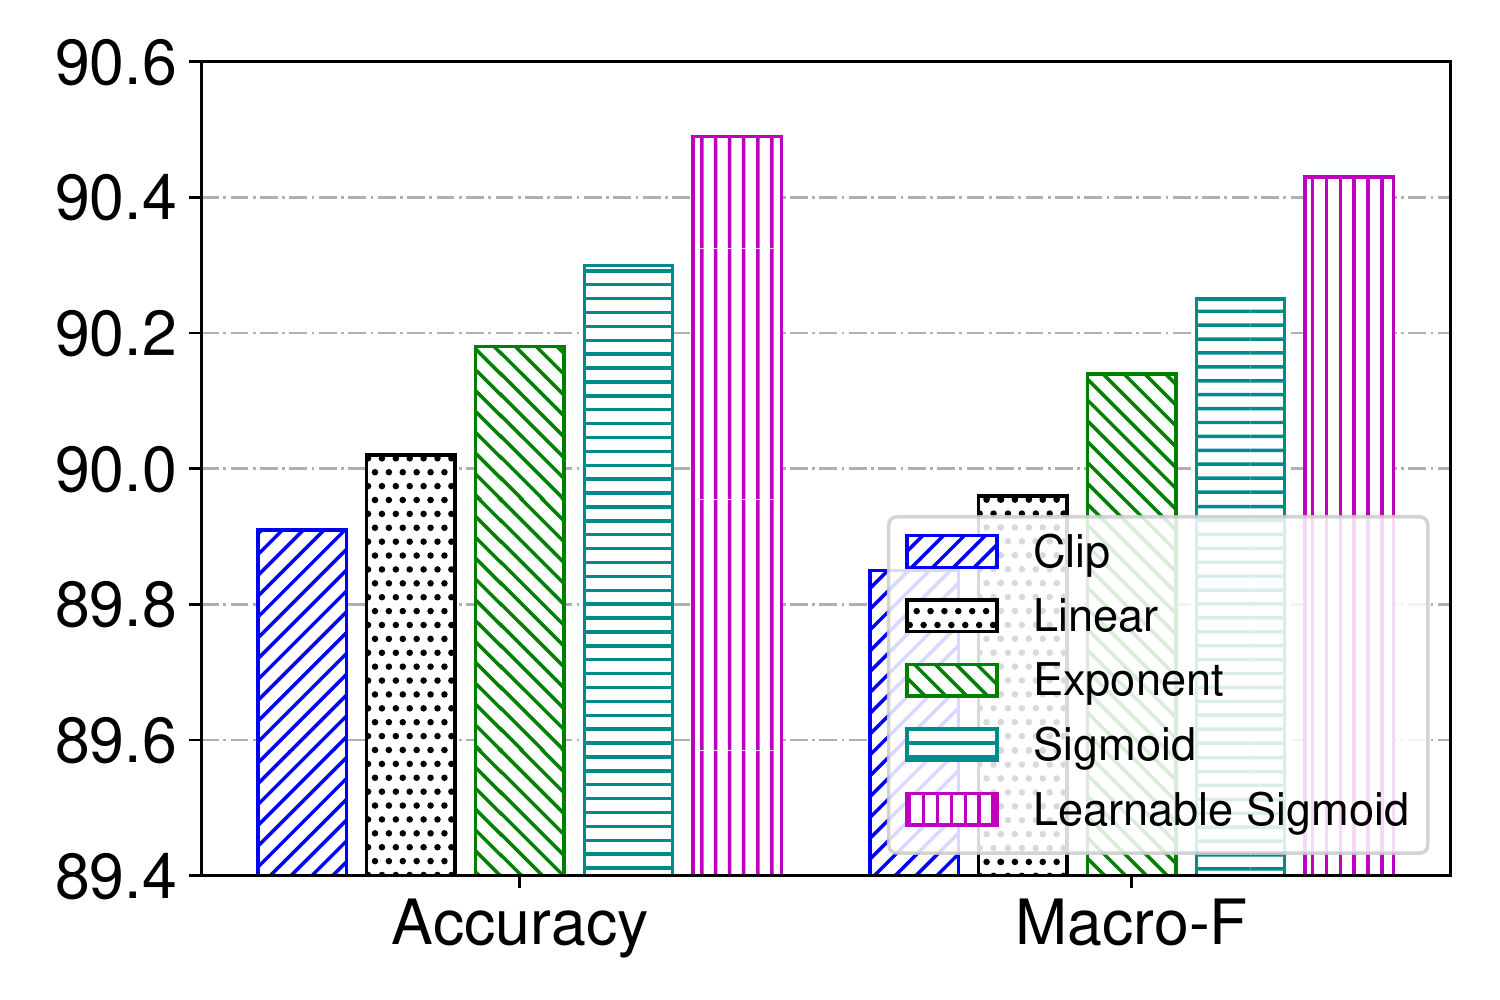} 
	}
		\subfigure[\textit{SNLI}.]{
	\includegraphics[height=1.5in]{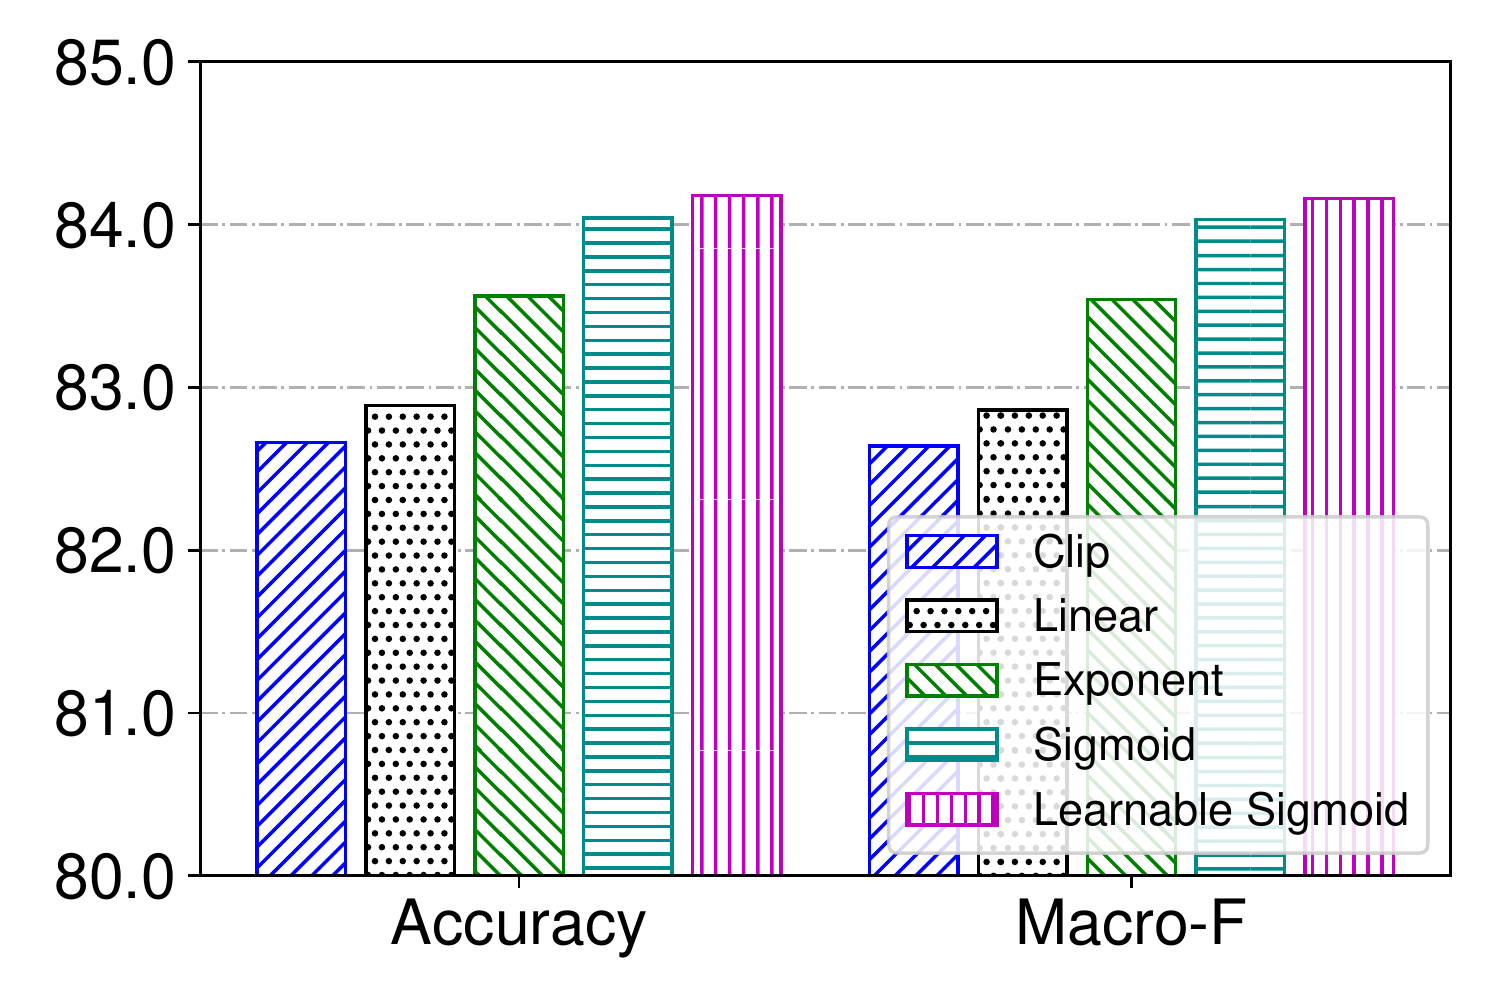} 
	} 
\caption{Influence of using different mapping functions on the \textit{SST} and \textit{SNLI} datasets.}\label{fig.positionfunc14}
\end{figure}

\begin{figure}[!t]
	\centering 
	\subfigure[\textit{SST}.]{
	\includegraphics[height=1.5in]{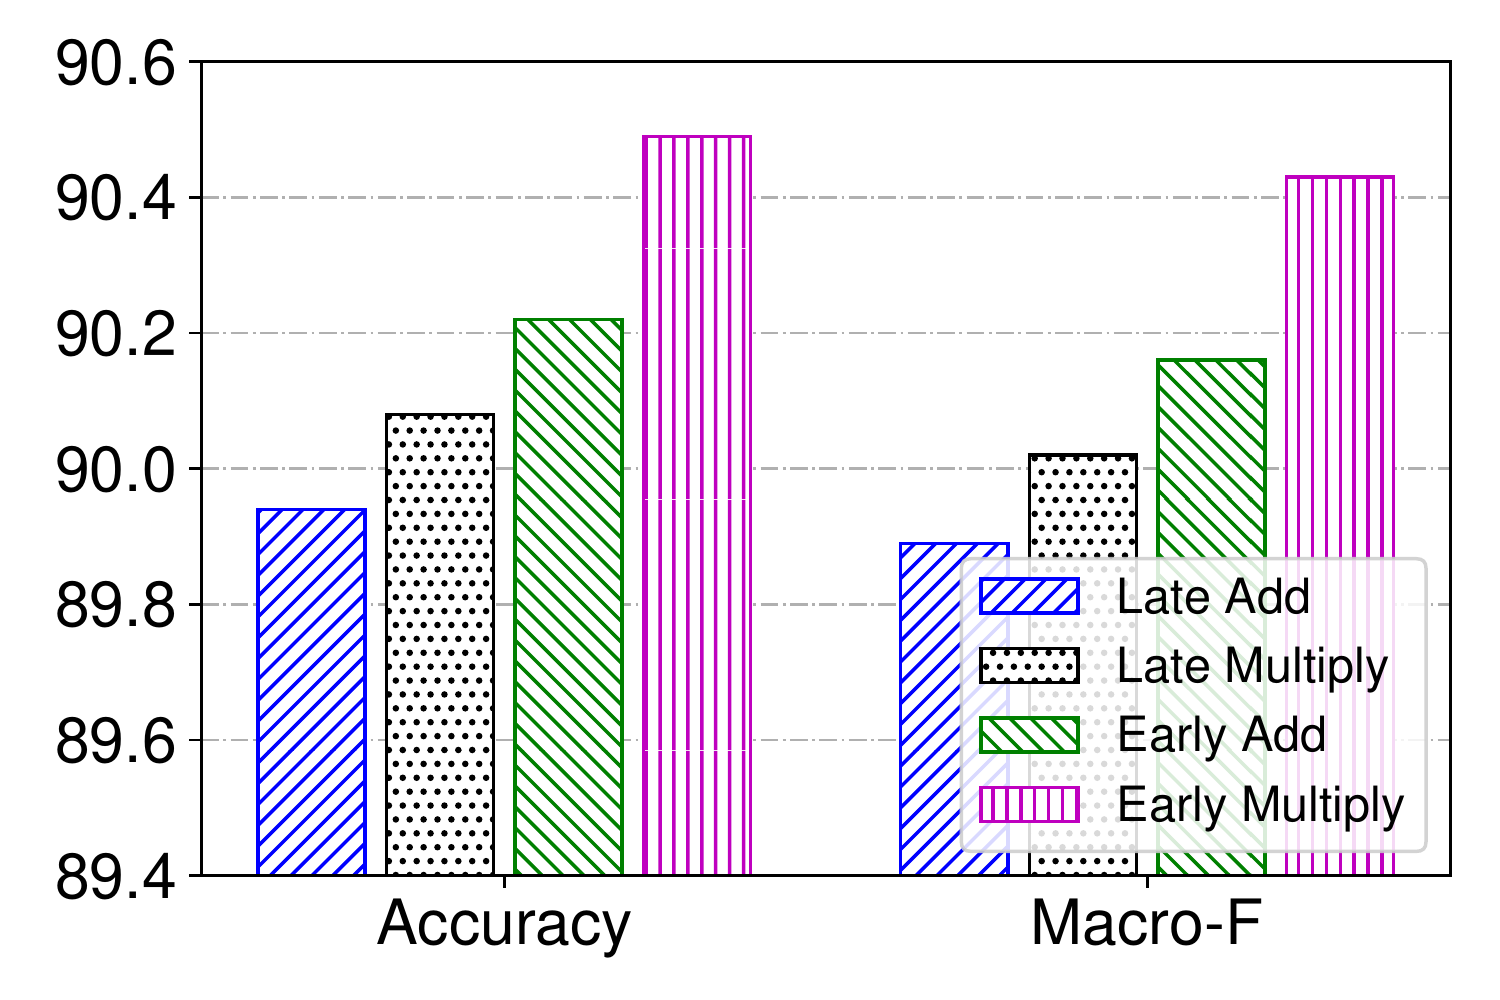} 
	}
		\subfigure[\textit{SNLI}.]{
	\includegraphics[height=1.5in]{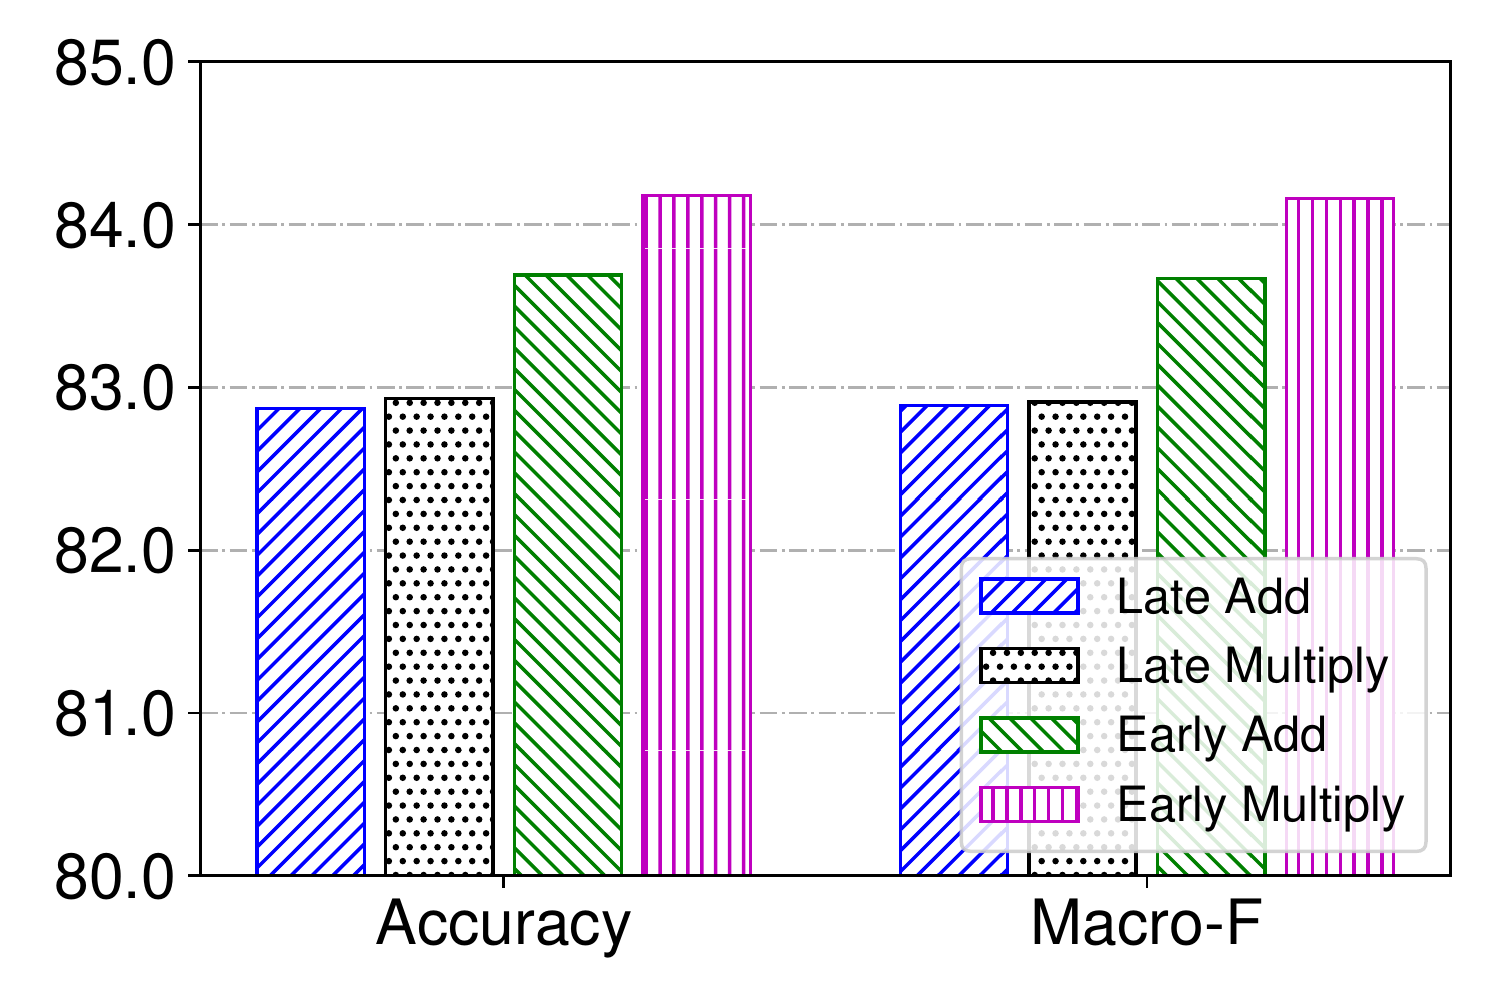} 
	}

\caption{Influence of using different attention adjusting methods on the \textit{SST} and \textit{SNLI} datasets.}\label{fig.positionfunc24}
\end{figure}

\begin{figure}[!t]
	\centering 
	\subfigure[\textit{SST}.]{
	\includegraphics[width=0.22\textwidth]{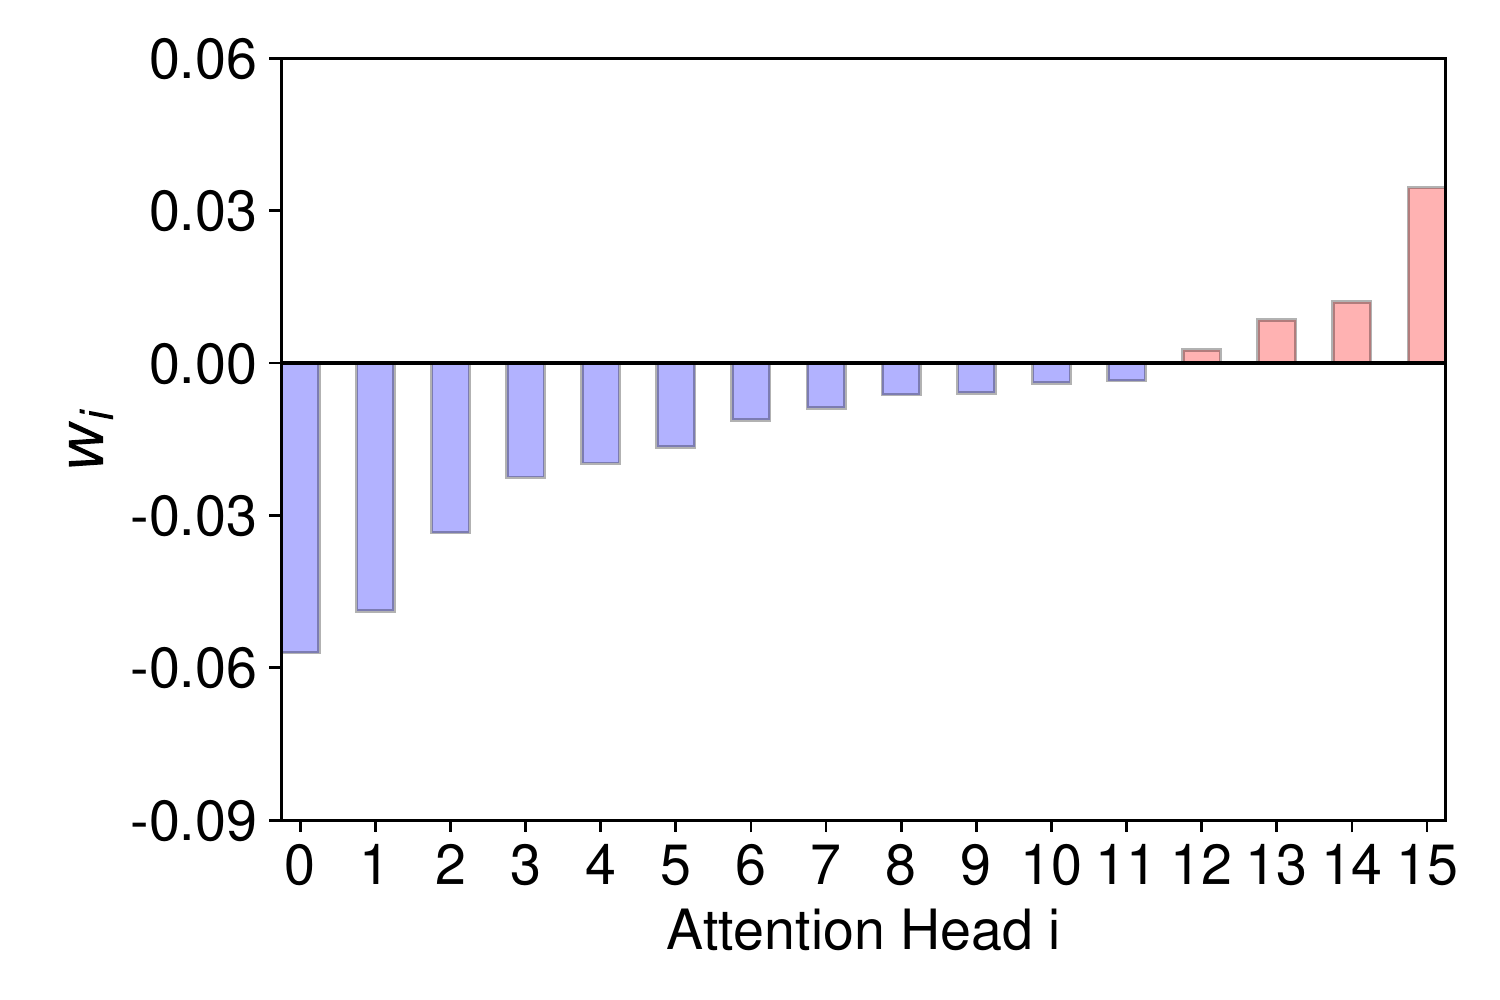} \label{fig.ssthead}
	}
		\subfigure[\textit{SNLI}.]{
	\includegraphics[width=0.22\textwidth]{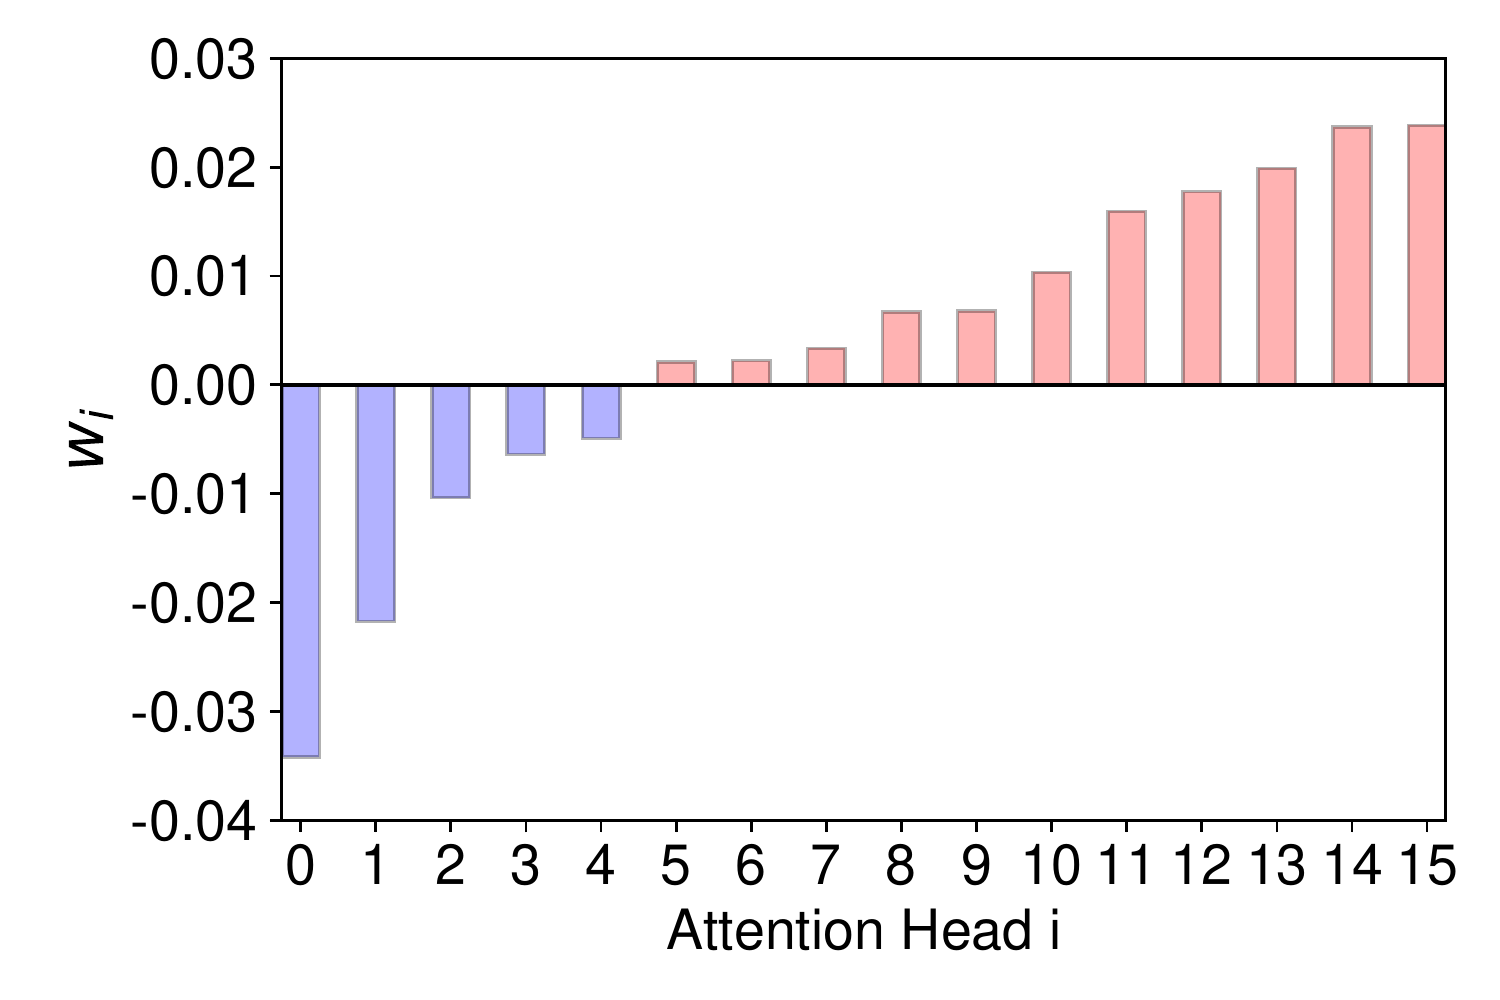} \label{fig.snlihead}
	}
\caption{The  distance weights learned by different attention heads on the \textit{SST} and \textit{SNLI} datasets.}\label{fig.sstsnlihead}
\end{figure}

\begin{figure}[!t]
	\centering 
	\subfigure[Word-level Transformer.]{
	\includegraphics[width=0.22\textwidth]{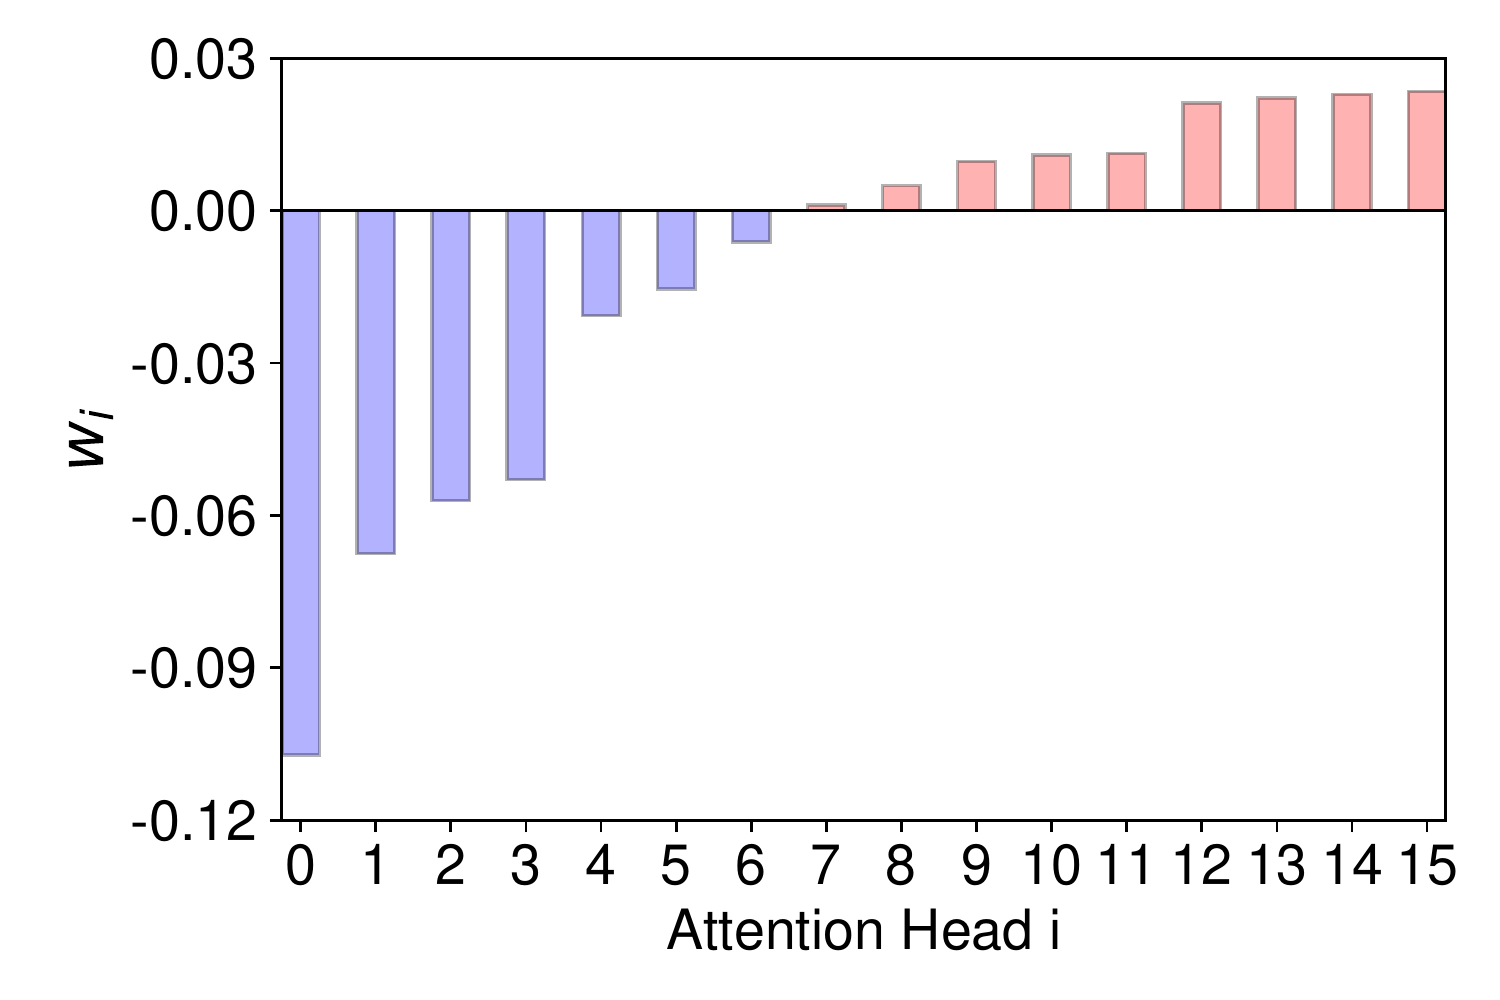} \label{fig.amazonhead1}
	}
		\subfigure[Sentence-level Transformer.]{
	\includegraphics[width=0.22\textwidth]{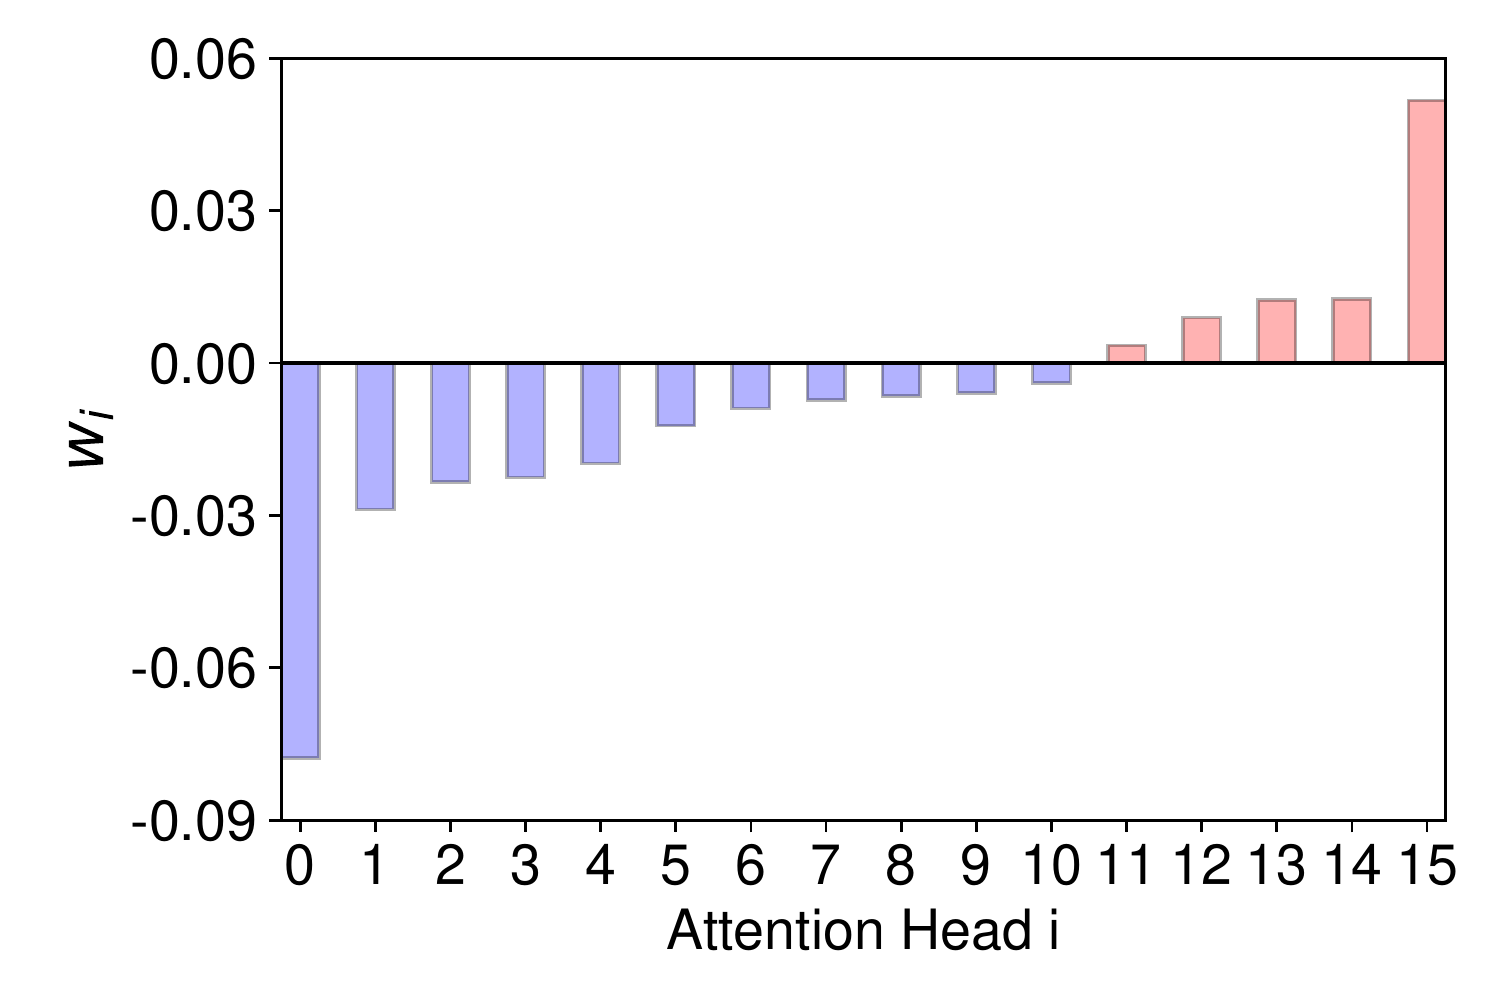} \label{fig.amazonhead2}
	}
\caption{The  distance weights learned by different attention heads on the \textit{Amazon} dataset.}\label{fig.amazonhead}
\end{figure}
